# Supplementary material for: Designing Flat Bands, Localized and Itinerant States in TaS2 Trilayer Heterostructures
Source: arXiv:2502.08793 source file (2025-02-12)
Supplement: Supplementary file 1 [file Supplementary.pdf]

# Supplementary Information

## 1. EFFECT OF $U$ ON CORRELATION-DRIVEN AND HYBRIDIZATION GAPS IN 1T-$TaS_2$

We demonstrate that the primary mechanisms driving gap opening in monolayer 1T-$TaS_2$ and bilayer T/T-$TaS_2$ are electronic correlation and orbital hybridization, respectively. Our analysis is based on DFT+U calculations, where we also examine a $U_{\mathrm{Ta,5d}} = 2.27$ eV, as suggested for bulk 1T-$TaS_2$ [1].

Fig. S1 illustrates the dependence of the band gap on $U$ for various 1T-$TaS_2$ systems. The monolayer exhibits distinct gap sizes that increase linearly with $U$, as shown in Figure S2(b). In contrast, for bilayer T/T-$TaS_2$, the band gap demonstrates only a minor increase from 308 to 340 meV in the $T_A$ stacking and 104 to 142 meV in the $T_B$ stacking. The contrasting trends between monolayer and bilayer indicate that the band gap in bilayer T/T-$TaS_2$ is predominantly governed by inter-SoD hybridization, rather than correlation effects within the SoD clusters.

Additionally, our calculations indicate that when a monolayer is stacked to form a bilayer ($T_A$ or $T_B$ stacking), the bandwidth of the lower flat bands decreases, as depicted in Fig. S2(a). The reduction in bandwidth suggests increased localization of the electronic states due to inter-SoD hybridization. Moreover, our analysis confirms the increased in-plane hopping components from $T_A$, to $T_B$, and $T_C$ enhance the band dispersions [2–4].

## 2. CHARGE TRANSFER IN THE TRILAYER T/T/H-$TaS_2$

To estimate the electron transfer from the T/T bilayer to the 1H monolayer in a T/T/H-$TaS_2$, we analyze the density of states (DOS) of the split flat band states. Fig. S3 illustrates how hole doping in the bilayer modifies the DOS and how electron transfer is computed.

To determine the amount of transferred charge, we integrate the DOS over the energy range corresponding to the split flat band states. The upper and lower bounds are defined by the stationary points in the DOS profile. Using this method, we estimate charge transfers of 0.80, 0.82, and 1.00 electrons for the $T_A$, $T_B$, and $T_C$ stacking orders, respectively.

We note that these values should be interpreted qualitatively, as they depend on the arbitrary choice of atomic radii in the projected DOS. For this analysis, we used 1.517 Å and 1.699 Å as the radii for Ta and S atoms based on our Bader charge analysis [6], respectively.

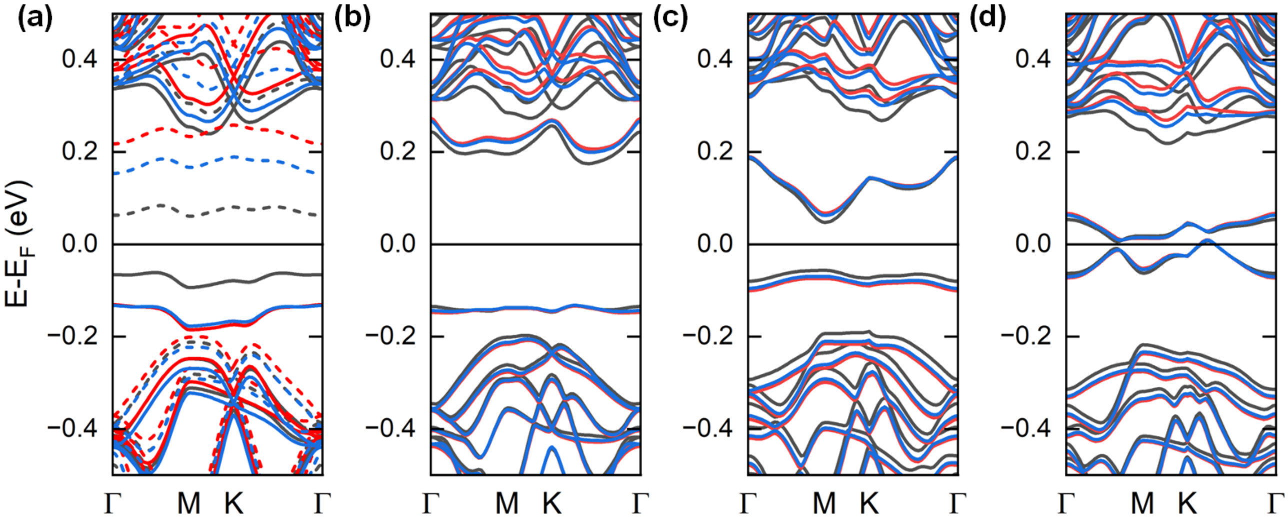


**Supplementary Figure 1: Band gap variation as a function of $U$ for monolayer and bilayer 1T-$TaS_2$.** Panels (a) and (b-d) illustrate the electronic band structures of (a) monolayer 1T-$TaS_2$ and (b-d) bilayer T/T-$TaS_2$ in the $T_A$, $T_B$, and $T_C$ stacking configurations, respectively. Black, blue, and red lines correspond to $U_{\mathrm{eff,1T}}$=0, 1.76 [5], and 2.27 eV [1], respectively. Majority and minority spins are denoted as a solid and dashed lines, respectively.

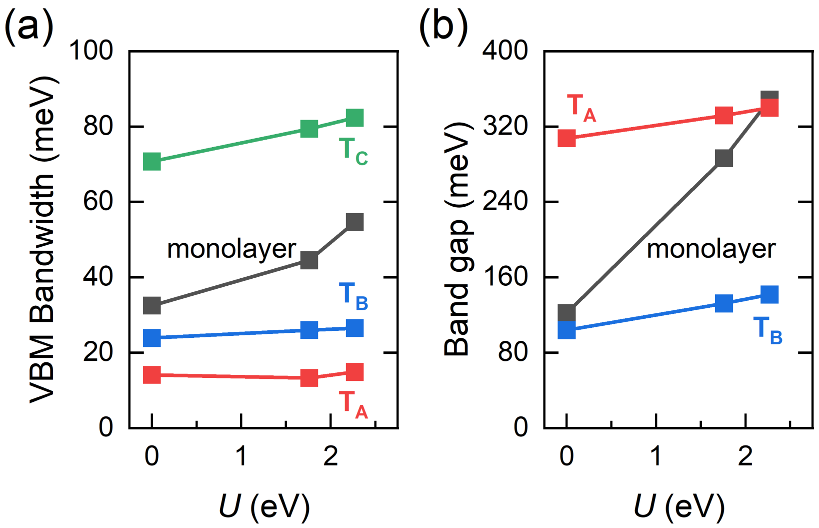


**Supplementary Figure** 2: **Dependence of flat band bandwidths and band gaps on $U$ in monolayer 1T-$TaS_2$ and bilayer T/T-$TaS_2$.** (a) Variation of the valence band maximum (VBM) bandwidths in the monolayer and bilayer systems as a function of $U$. (b) Corresponding band gap evolution extracted from Fig. S1.

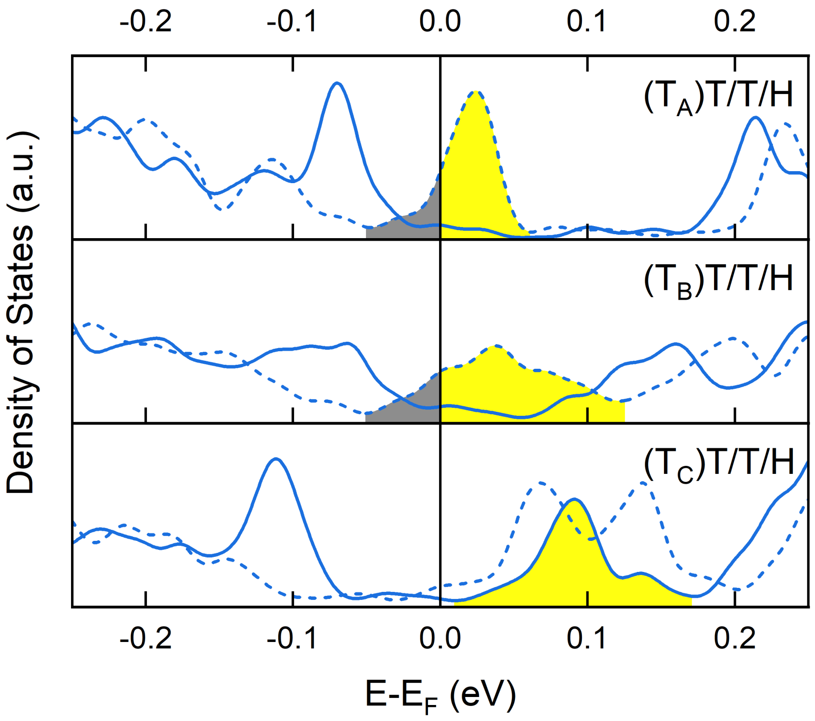


**Supplementary Figure** 3: **Electron transfer from the T/T bilayer to 1H layer in a T/T/H trilayer, depending on the stacking configuration of the T/T bilayer.** Each panel presents the DOS projected onto the T/T bilayers for the $T_A$ (top), $T_B$ (middle), $T_C$ (bottom) stacking orders. Solid and dashed lines denotes majority and minority spins, respectively. The yellow-shaded area represents unoccupied states, indicating the fraction of transferred electrons. Charge transfer is estimated by integrating the split flat band DOS, assuming full occupancy corresponds to one electron.

[1] P. Darancet, A. J. Millis, and C. A. Marianetti, Physical Review B **90**, 045134 (2014).

[2] T. Ritschel, J. Trinckauf, K. Koepernik, B. Büchner, M. v. Zimmermann, H. Berger, Y. Joe, P. Abbamonte, and J. Geck, Nature physics **11**, 328 (2015).

[3] T. Ritschel, H. Berger, and J. Geck, Physical Review B **98**, 195134 (2018).

[4] J. M. Pizarro, S. Adler, K. Zantout, T. Mertz, P. Barone, R. Valentí, G. Sangiovanni, and T. O. Wehling, npj quantum materials **5**, 79 (2020).

[5] C. G. Ayani, M. Bosnar, F. Calleja, A. P. Solé, O. Stetsovych, I. M. Ibarburu, C. Rebanal, M. Garnica, R. Miranda, M. M. Otrokov, *et al.*, Nano Letters **24**, 10805 (2024).

[6] W. Tang, E. Sanville, and G. Henkelman, Journal of Physics: Condensed Matter **21**, 084204 (2009).
